# Supplementary material for: Combining the Ensemble and Franck-Condon Approaches for Spectral Shapes of Molecules in Solution
Source: arXiv:1709.07490 ancillary file (2017-09-27)
Supplement: Supplementary file 1 [file supporting_info.pdf]

# Supporting information for *"Combining the Ensemble and Franck-Condon Approaches for Spectral Shapes of Molecules in Solution"*

T. J. Zuehlsdorff[1,*] and C. M. Isborn[1,†]

[1] *School of Natural Sciences, University of California Merced, N. Lake Road, CA 95344, USA*

(Dated: September 21, 2017)

*Electronic address: tzuehlsdorff@ucmerced.edu

†Electronic address: cisborn@ucmerced.edu

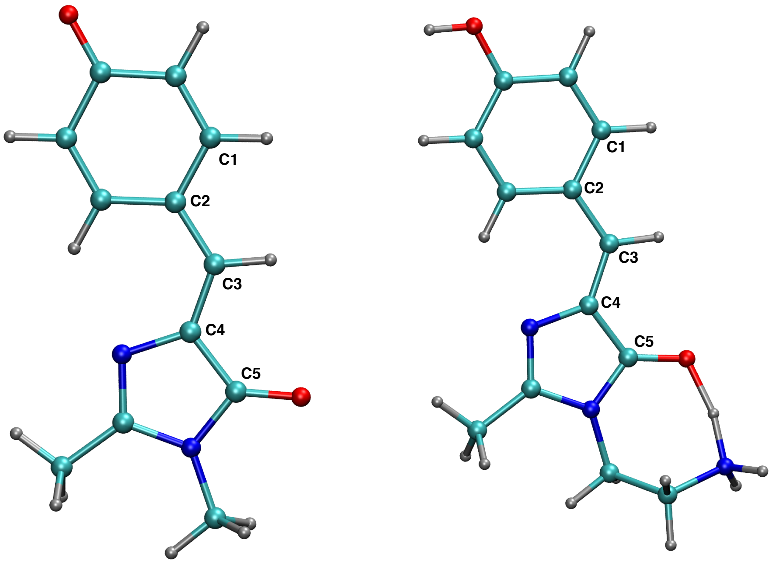


a) GFP anion  b) GFP neutral+

FIG. 1: Ball and stick representation of the ground state structure of GFP anion and neutral+. The dihedral angles that are reparameterized from the standard AMBER values are defined through C1-C2-C3-C4 and C2-C3-C4-C5. This figure was created using VMD [4].

## I. THE AMBER FORCE FIELD

A key ingredient for the modeling of absorption spectra of solvated dyes is the generation of a representative sample of solute-solvent conformations that are used to compute the vertical excitation energies. In this work, we use the generalized AMBER force field[1] to describe the three chromophores, as well as the solvent molecules of methanol, acetone, benzene, and cyclohexane, whereas water is described by the TIP3P model[2]. For the chromophores, the force field parameters of some of the most important degrees of freedom are then individually checked against scans of the DFT B3LYP[6]/6-41+G* potential energy surface and are, if necessary, reparameterized. For Nile Red, the standard force field is reparameterized following the Supporting Information of Ref. [3] to better describe rotations around the C-N bond that connects the conjugated system to the diethylamino group.

For the GFP chromophores, we focus on the dihedral angles describing the orientation of the conjugated backbone of the molecules (see Fig. 1), as they are expected to have a strong influence on the bright low-energy excited states of interest. We therefore perform a scan of the potential energy surface along the rotation around both dihedral angles for

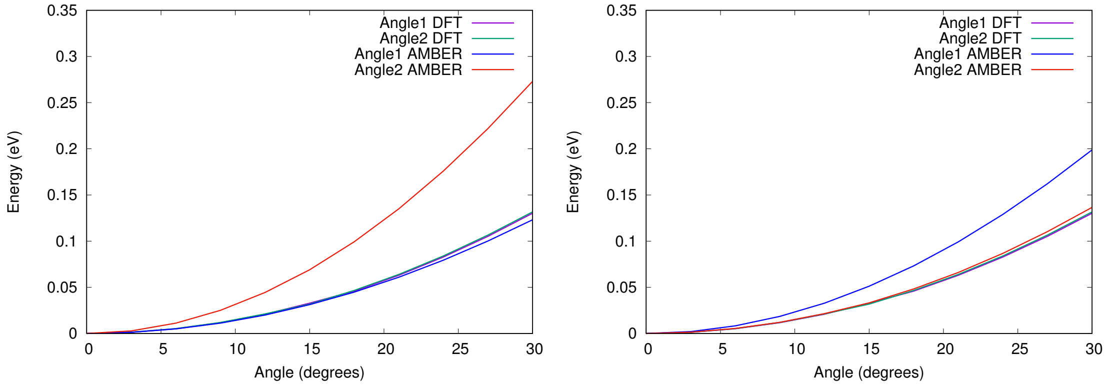


a) Standard AMBER parameters  b) Reparameterised AMBER

FIG. 2: Potential energy surface of twisting the GFP anion around Angle1= C1-C2-C3-C4 and Angle2=C2-C3-C4-C5, as calculated using DFT at the B3LYP/6-31+G* level. Furthermore, the AMBER potential energy surfaces as calculated for the optimized DFT geometries along the twist path are also displayed, once before reparameterizing the dihedral force constants of the two angles and once after.

the GFP anion in vacuum using the Gaussian code[5]. The calculations are performed at the B3LYP[6]/6-31+G* level of theory and the twist angle is increased in increments of 3° from its ground state configuration, while a full geometry optimization of all other degrees of freedom is carried out at each step. We then take the optimized geometries along the DFT twist path for each dihedral angle and compute AMBER energies for the structures using the standard AMBER force field. The results of the calculation can be found in Fig. 2.

As can be seen, the DFT scan predicts that the potential energy barrier encountered when twisting the molecule out of its planar conformation is the same for both dihedral angles, while the AMBER force field predicts a much larger energy barrier for angle 2 than for angle 1. The reason for this can be straightforwardly understood by considering that AMBER assigns a double-bond character to the C3-C4 bond and a single-bond character to the C2-C3 bond, while in DFT both bonds show shared characteristics. Thus in the standard AMBER force field, any out-of-plane distortion to the GFP molecule will preferentially occur around the dihedral angle 1, rather than be shared equally between the two angles.

To address the shortcomings of the AMBER force field we assign the same dihedral force constant to both angles and fit its value to the DFT potential energy scan. The results

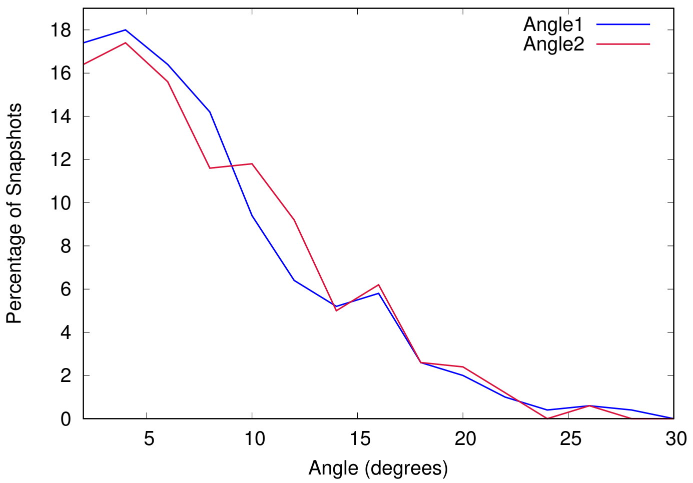


FIG. 3: Histogram of dihedral angles 1 and 2 of the GFP anion in vacuum, as calculated from a 4 ns MD trajectory sampled at 4 ps intervals, where the reparameterized AMBER force field is used to compute the trajectory.

can be found in Fig. 2. As can be seen, while the reparameterization using a single force constant for both dihedral angles does not yield an identical potential energy barrier for the minimum energy twist path derived from DFT, the error of the standard force field is significantly reduced. For the purpose of this work, which aims at producing a set of realistic solvent-solute conformations rather than highly accurate dynamics, the reparameterization of the dihedral angles is considered sufficient and the same force constant is also used for the GFP neutral+ chromophore.

To confirm that the remaining discrepancy in potential energy barriers for the two dihedral angles in the reparameterized AMBER force field does not give rise to preferentially twisted conformations, we compute the histogram of both dihedral angles for 1000 snapshots taken from a 4 ns MD trajectory of the GFP anion in vacuum at 300 K. The results are displayed in Fig. 3. As can be seen, the GFP molecule stays preferentially in a flat conformation and both dihedral angles produce a very similar angular distribution, suggesting that the chosen reparameterization of the AMBER force field is sufficient to prevent preferential twists around one of the two dihedral angles.

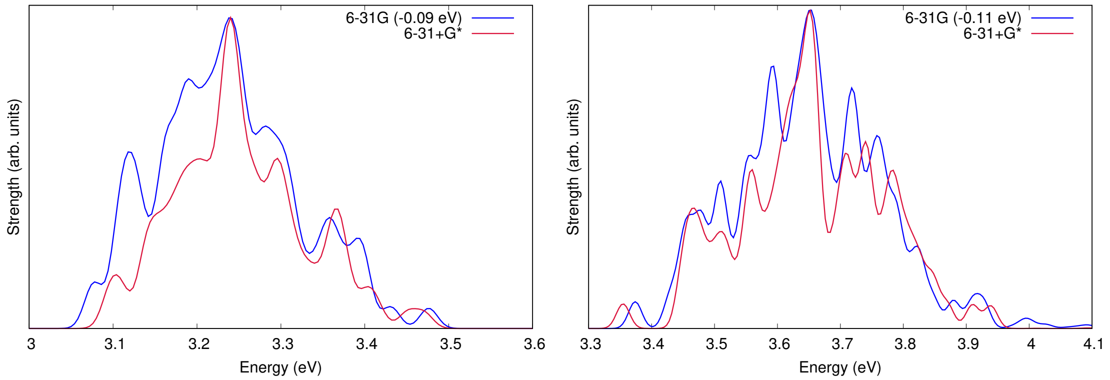


a) GFP anion in water

b) GFP neutral+ in methanol

FIG. 4: Vertical absorption spectra for GFP anion in water and neutral+ in methanol, as calculated for 100 MD snapshots, with a 6-31G and a 6-31+G* Gaussian basis set. A Gaussian broadening with $\sigma = 0.0105$ eV is applied to both spectra.

## II. VERTICAL EXCITATION ENERGIES

In this section, we examine the sensitivity of vertical excitation energies computed from the AMBER MD trajectories with respect to the choice of basis set, as well as the size of the QM region used to represent the solvent environment. All calculations are performed using TeraChem[7, 8] and the CAM-B3LYP functional[9]. The Tamm-Dancoff approximation[10, 11] is applied throughout.

### A. Basis set

First, we focus on the two GFP chromophores in solution and compare excitation energies obtained from a 6-31G basis set to those computed with a 6-31+G* basis set. To do so, we take the first 100 uncorrelated MD snapshots of both systems, where the QM region was chosen to include all solvent molecules with a center of mass within 8 Å of any solute atom and all other solvent molecules are included in the calculation as point charges. A Gaussian broadening with $\sigma = 0.0105$ eV is applied to the excitation energies and the resulting spectra can be found in Figure 4. Given the relatively small number of snapshots considered for the convergence test, the spectra are considerably less smooth than those obtained for the full set of 2000 uncorrelated snapshots presented in the main manuscript. However, it can be

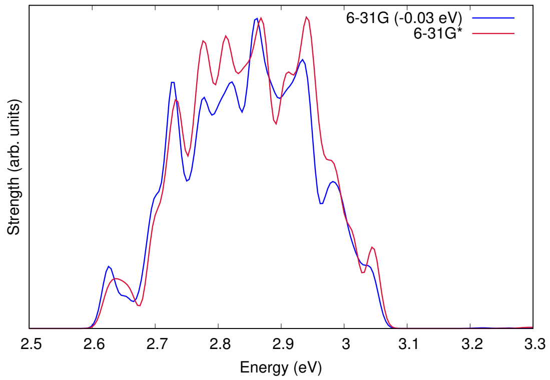


a) Nile Red in acetone

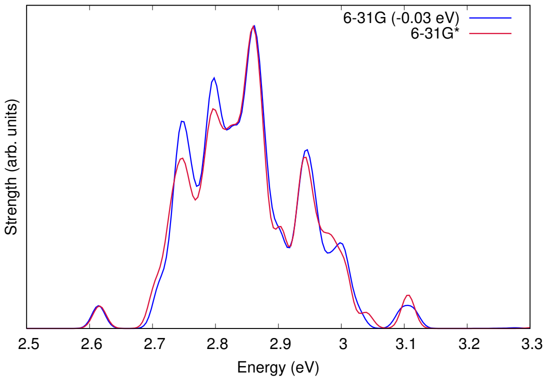


b) Nile Red in benzene

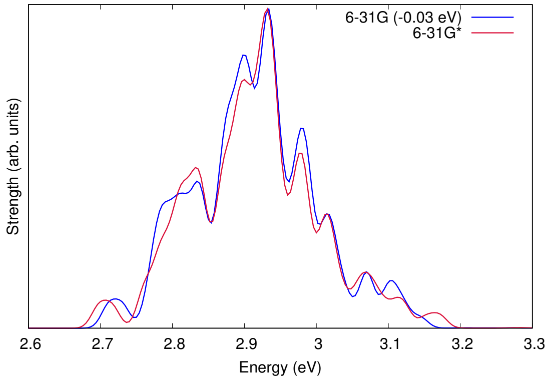


c) Nile Red in cyclohexane

FIG. 5: Vertical absorption spectra for Nile Red in acetone, benzene and cyclohexane, as calculated for 100 MD snapshots, with a 6-31G and a 6-31G* Gaussian basis set. A Gaussian broadening of $\sigma = 0.0105$ eV is applied to all spectra.

seen that the larger basis set causes a significant red-shift of both spectra, while its width stays relatively constant.

We repeat the above calculations for Nile Red in acetone, benzene, and cyclohexane, with the difference that we compare the 6-31G basis set to the 6-31G* basis set in order to avoid numerical issues caused by the diffuse functions for a number of snapshots of Nile Red in acetone. The results can be found in Fig. 5 and again show that although the larger basis set causes a red-shift of the spectrum of vertical excitation energies, the shape and the width are relatively uninfluenced.

Although it is unsurprising that the small 6-31G basis set does not yield converged excitation energies for the dyes in question, with the absolute energies of the GFP anion

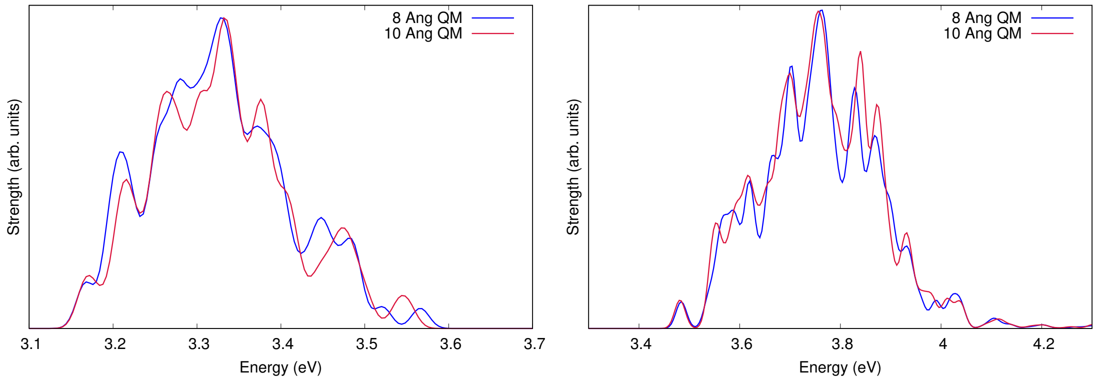


a) GFP anion in water

b) GFP neutral+ in methanol

FIG. 6: Vertical absorption spectra for GFP anion in water and neutral+ in methanol, as calculated for 100 MD snapshots for two different QM region sizes. For the first data set, all solvent molecules whose center of mass is within 8 Å of any solute atom are treated quantum mechanically, whereas for the second set, the cutoff distance is increased to 10 Å. A Gaussian broadening with $\sigma = 0.0105$ eV is applied to both spectra.

being particularly influenced as already noticed by other researchers[12], we point out that the main focus of our work is to correctly reproduce the width and shape of absorption spectra. Given how well these properties of interest are captured by the small 6-31G basis set and given the large number of TDDFT calculations required in this work, we limit ourselves to the 6-31G basis set for the computation of all vertical excitation energies in the systems studied.

### B. QM region size

We next focus on the convergence of the vertical excitation energies of the solvated systems with respect to the QM region size. For this purpose, we perform calculations on the first 100 MD snapshots of the full 8 ns trajectory, where the QM region is limited to all solvent molecules with a center of mass that is within 8 Å and 10 Å of any solute atom. The 8 Å cutoff radius yields QM region sizes of $\approx$ 550-600 atoms, whereas for the 10 Å cutoff the number of atoms explicitly treated quantum mechanically in the TDDFT calculation is $\approx$ 850-900. All calculations are performed at the CAM-B3LYP/6-31G level of theory.

The results for the GFP anion in water and GFP neutral+ in methanol can be found

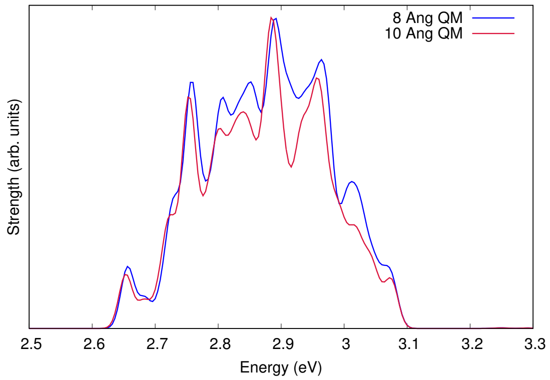


a) Nile Red in acetone

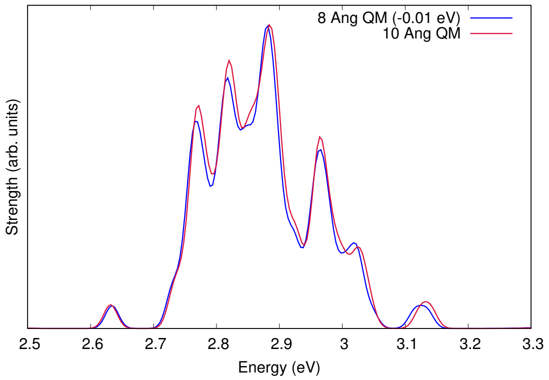


b) Nile Red in benzene

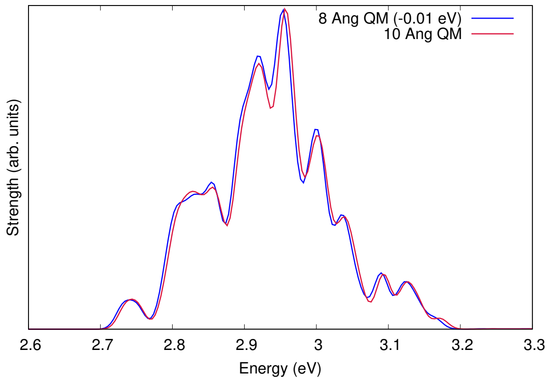


c) Nile Red in cyclohexane

FIG. 7: Vertical absorption spectra for Nile Red in acetone, benzene and cyclohexane, as calculated for 100 MD snapshots for two different QM region sizes. For the first data set, all solvent molecules whose center of mass is within 8 Å of any solute atom are treated quantum mechanically, while for the second set, the cutoff distance is increased to 10 Å. A Gaussian broadening with $\sigma = 0.0105$ eV is applied to all spectra.

in Fig. 6, the results for Nile Red in acetone, benzene, and cyclohexane are presented in Fig. 7. All spectra are shifted and scaled to have the same height. As can be seen, both the shape and the width of the vertical absorption spectra are well converged with respect to the size of the QM region for the 8 Å cutoff radius. The largest discrepancies are found for Nile Red in acetone and the GFP anion in water, but are significantly smaller than the discrepancies introduced by varying the basis set size. For the purpose of this work, the QM region using an 8 Å cutoff radius is therefore considered to be sufficient to fully capture the influence of solvent polarization on the shape of the vertical absorption spectrum.

## III. VIBRONIC SHAPE FUNCTIONS

The final key ingredient to computing optical absorption spectra of solvated dyes as proposed in this work is the vibronic shape function. In this section, we study the effects of basis set size, chosen DFT functional, finite temperature effects, as well as the inclusion of explicit solvent representations on the computed shape functions in order to assess their reliability in correctly describing the vibronic fine structure of the excitation of interest. Throughout this section, unless specified otherwise, solvent effects on the vibronic spectra are accounted for by using an implicit solvent model. Unless further specified, all spectra are computed at the CAM-B3LYP/6-31G level of theory at a temperature of 0 K using Gaussian[5], and the Tamm-Dancoff approximation is applied throughout.

### A. Basis set

We first assess the convergence of the vibronic shape functions with the size of the basis set used for all three chromophores. Specifically, we compare the spectra for the GFP anion in water, GFP neutral+ in vacuum, and Nile Red in acetone using both the 6-31G and the 6-31+G* basis set. The reason why the comparison for GFP neutral+ is performed in vacuum, is that for certain implicit solvent environments and basis sets the optimized $S_1$ geometry of the GFP chromophore corresponds to a structure that is twisted out of plane. This significantly reduces the overlap of the ground state and excited state nuclear wave functions, leading to a breakdown of the Franck-Condon principle, which results in an unreliable vibronic spectrum. Note that this issue has only been encountered for the GFP chromophore in implicit solvent and not in the frozen explicit solvent environments and thus does not influence the shape functions that are used for calculating vibronically broadened absorption spectra in this work.

The basis set dependence of the vibronic spectra of all three dyes is displayed in Fig. 8. As can be seen the smaller 6-31G basis set correctly captures the general shape of the vibronic spectra for all three solvents, including the relative positions of the main peaks. For Nile Red, the agreement between the 6-31+G* and the 6-31G basis sets is very good, whereas for GFP neutral+ there is a minor change in the relative intensity of the two secondary peaks. For the GFP anion, the basis set dependence of the vibronic spectrum is somewhat stronger,

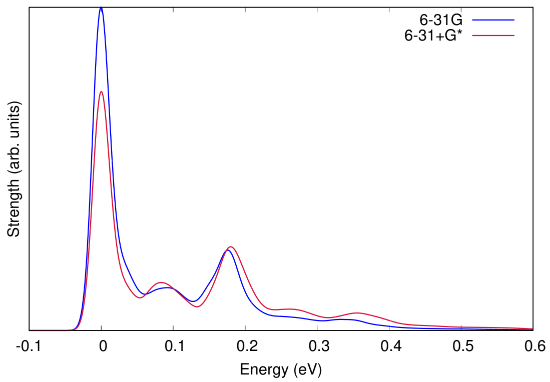


a) GFP anion in water

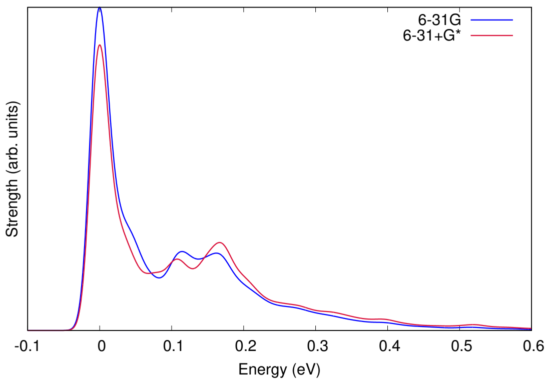


b) GFP neutral+ in vacuum

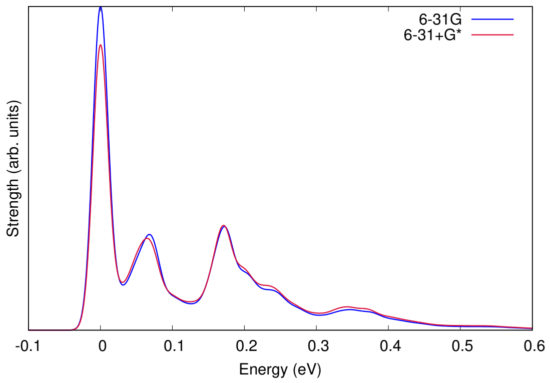


c) Nile Red in acetone

FIG. 8: Vibronic shape functions for GFP anion in water, GFP neutral+ in methanol and Nile Red in acetone, as calculated in the implicit solvent model. One set of results is computed using a 6-31G basis set, while the other is computed using the 6-31+G* basis set. All spectra are shifted such that the 0-0 peak is at 0 eV. A Gaussian broadening with $\sigma = 0.0105$ eV is applied to all shape functions.

in agreement with previous work[13], where a 6-31G* basis set was recommended to capture the main features of the vibronic spectrum. Given that the overall shape and width of the spectra for the GFP neutral+ chromophore and Nile Red is well reproduced by the smaller 6-31G basis set, and given the computational cost of performing excited state frequency calculations of the dyes in explicit frozen solvent environment, we limit all calculations of the vibronic shape functions for these systems to the smaller basis set, while the GFP anion shape functions are computed using the larger 6-31+G* basis set.

### B. DFT functional

In this work, we make use of the standard CAM-B3LYP functional throughout, both for the computation of vibronic shape functions and the vertical excitation energies. This is motivated by the fact range-separated hybrids such as CAM-B3LYP have been shown to yield good results for the $S_1$ potential energy surface of Nile Red when compared to other DFT functionals[14] and ab-initio methods[15]. In order to test the effect varying the exchange correlation functional on the computed vibronic shape functions, we calculate the shape functions for the GFP anion in water, GFP neutral+ in methanol, and Nile Red in acetone using the $\omega$B97X functional, a range-separated hybrid functional that, unlike CAM-B3LYP, has the correct long-range limit[16].

Figure 9 shows the vibronic shape functions as calculated with the $\omega$B97X and the CAM-B3LYP functional. As can be seen, the results show some discrepancies in the predicted vibronic shape functions depending on the DFT functional used, which are especially prominent for the Nile Red chromophore. The $\omega$B97X functional predicts considerably broader vibronic spectra than CAM-B3LYP in the case of Nile Red, suggesting that significant amount of spectral weight is shifted from the 0-0 transition to higher energy vibronic states.

The discrepancies in the vibronic shape functions for different DFT functionals are not fully surprising. The vibronic spectra are constructed from the Hessians of the ground and excited state potential energy surfaces around their respective minima and thus depend on the second derivative of the energy with respect to spatial coordinates. Therefore, relatively small changes in the excitation energies can have a significant influence on the vibronic spectra.

The results shown here suggest that the choice of DFT functional can have a significant influence on the vibronic spectra of small chromophores and that, where possible, such choice should be informed by comparing the potential energy surfaces along important vibrational modes to ab-initio quantum chemistry methods. For the purpose of this work we refer to existing literature for a demonstration of the suitability of the CAM-B3LYP functional in describing important features of the $S_1$ potential energy surface of the Nile Red chromophore[14]. For the GFP chromophores, we note that the sensitivity with respect to the exchange-correlation functional is considerably less pronounced. Furthermore, for the GFP anion, a previous study has been carried out[13] where the Franck-Condon spectrum of

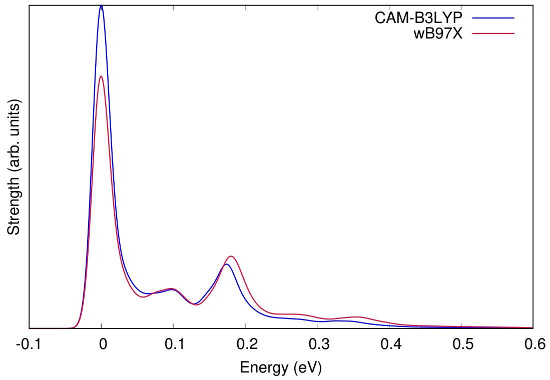


a) GFP anion in water

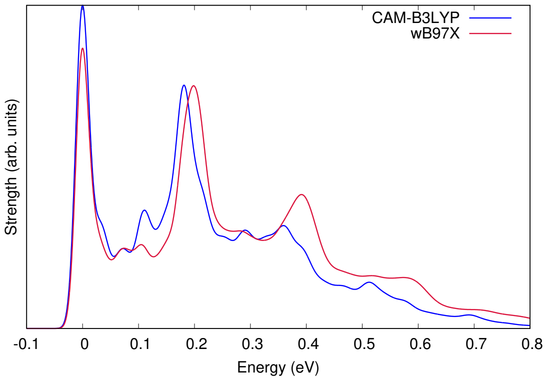


b) GFP neutral+ in methanol

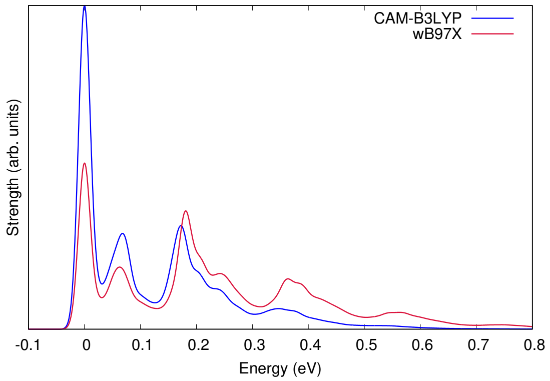


c) Nile Red in acetone

FIG. 9: CAM-B3LYP and $\omega$B97X vibronic shape functions for GFP anion in water, GFP neutral+ in methanol and Nile Red in acetone, as calculated in the implicit solvent model. All spectra are shifted such that the 0-0 peak is at 0 eV. A Gaussian broadening with $\sigma = 0.0105$ eV is applied to all shape functions.

CAM-B3LYP was found to be in good agreement with CASPT2 and XMCQDPT2 results. We therefore use the CAM-B3LYP functional for all vibronic spectra reported in this work.

### C. Temperature dependence

The vibronic functions used in constructing the absorption spectra of the chromophores chosen for this work are all computed by applying the zero temperature approximation to the Franck-Condon spectra. The approximation assumes that only the ground state vibrational mode of the ground state potential energy surface is initially occupied when computing the

Franck-Condon overlaps, broadening due to temperature is accounted for fully classically. Implicitly, the treatment assumes that higher energy vibrational modes only account for a broadening of the vibronic spectrum, but do not significantly alter its main spectral features. In order to check the validity of the approximation we repeat the calculation of the Franck-Condon spectra for the GFP anion in water, GFP neutral+ in methanol and Nile Red in Acetone using the FCclasses code[17, 18], which allows for the inclusion of temperature effects by assuming a Boltzmann distribution of initial vibrational modes[19]. All spectra are simulated at a temperature of 300 K and compared with spectra generated under the zero temperature approximation.

Figure 10 shows the resulting spectra as computed with the FCclasses code. As can be seen, the full finite temperature treatment only introduces minor changes to the computed vibronic spectra in form of a slight broadening. The largest discrepancy can be found for GFP neutral+, where the zero temperature approximation leads to a slight decrease in intensity for the second most dominant peak in the spectrum. However given the small changes made to the spectrum at T=300 K, we can conclude that the zero temperature approximation that the ground state vibrational mode is exclusively occupied initially recovers all relevant vibronic features of the system.

### D. Explicit solvent effects

Finally, we consider the effect of including explicit solvent in the computation of the vibronic shape functions. Although implicit solvent models are expected to capture average polarization effects through the surrounding medium, direct solute-solvent interactions, such as hydrogen bondings between the GFP anion and water cannot be accurately resolved without some explicit solvent representation. To sample different solute-solvent conformations, five snapshots are averaged to produce an average vibronic shape function in solution. To make the computation of the vibronic spectra feasible, only the few solvent molecules closest to the chromophore are retained in the QM region, such that the total QM region size is between 80 and 130 atoms. Long range solvent effects are accounted for by an implicit solvent model. All explicit solvent molecules are kept frozen in the computation of the vibrational modes of the solute and dispersion effects are included through the Grimme empirical dispersion scheme[20]. Thus the calculations capture the effects of the explicit solvent

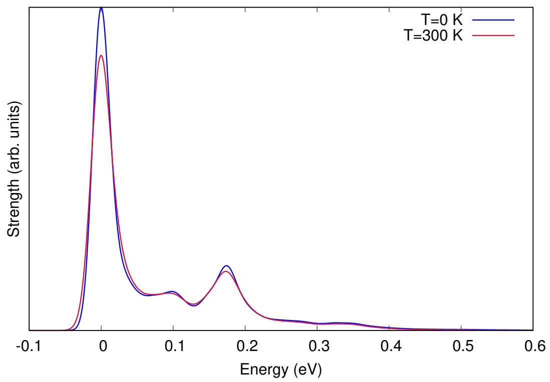


a) GFP anion in water

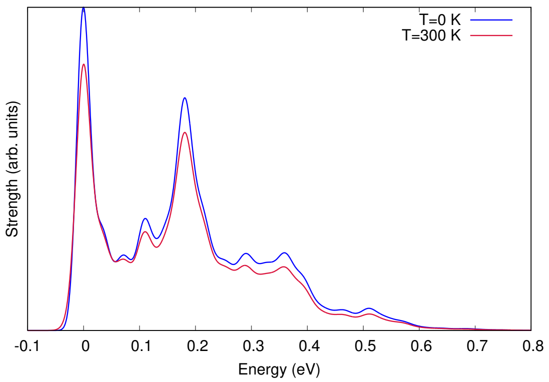


b) GFP neutral+ in methanol

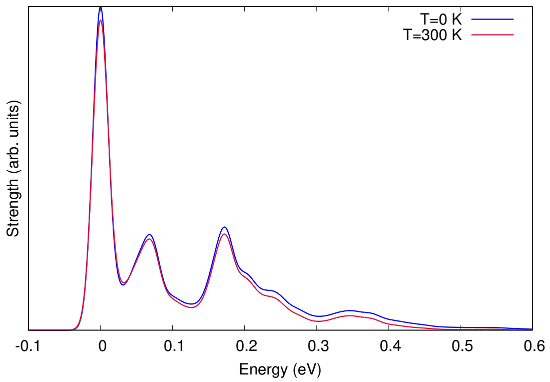


c) Nile Red in acetone

FIG. 10: Vibronic shape functions for GFP anion in water and GFP neutral+ in methanol and Nile Red in acetone, as calculated in the implicit solvent model. One set of results is computed in the zero temperature approximation, whereas the other set of results assumes a Boltzmann-weighted distribution of initial vibrational states to model a temperature of 300 K. All spectra are shifted such that the 0-0 peak is at 0 eV. A Gaussian broadening with $\sigma = 0.0105$ eV is applied to all shape functions.

environment on the solute electronic states but do not allow for a coupling to vibrational modes of the solvent. All calculations on nile red and the GFP neutral+ chromophore are performed at the CAM-B3LYP/6-31G level of theory, while for the GFP anion the 6-31+G* basis set is used.

The results for the GFP chromophores in solution are displayed Fig. 11, the ones for Nile Red are shown in Fig. 12. As can be seen, the general shape of the vibronic spectra, the position of vibronic peaks and their relative height, is relatively consistent between

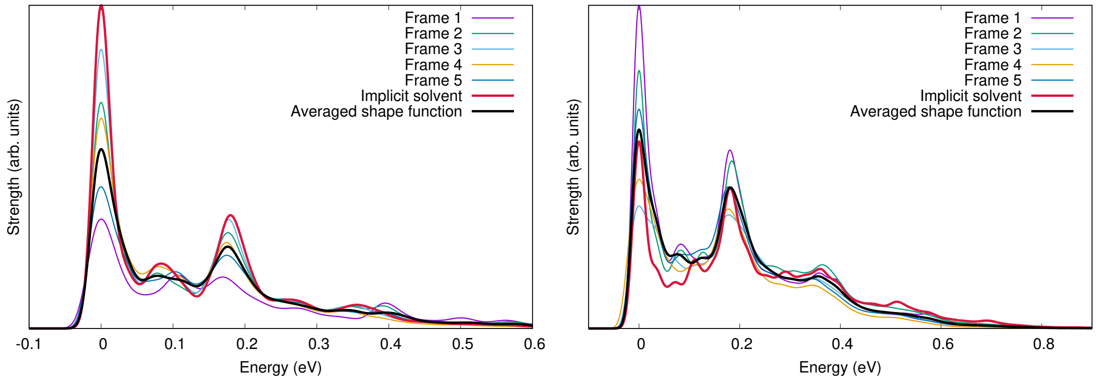


a) GFP anion in water

b) GFP neutral+ in methanol

FIG. 11: Vibronic shape functions for GFP anion in water and neutral+ in methanol, as calculated in implicit solvent as well as in frozen solvent environments taken from five uncorrelated MD snapshots. The vibronic shape function to used construct the absorption spectrum is the average of the vibronic spectra from the five individual frozen solvent snapshots and is also plotted for comparison. All spectra are shifted such that the 0-0 peak is at 0 eV. A Gaussian broadening with $\sigma = 0.0105$ eV is applied to all shape functions.

different explicit solvent snapshots. This confirms that constructing one average vibronic shape function for each system is a valid way of capturing explicit solvent effects. However, it is also noted that the GFP anion in water and the GFP neutral+ variant in methanol show considerably more variety between different solvent conformations than Nile Red in acetone or benzene. Furthermore, for the Nile Red chromophore in the three chosen solvents, the averaged vibronic shape function is similar to that computed in implicit solvent, however, this is not the case for the GFP anion, where the vibronic shape function derived from explicit solvent conformations has significantly more spectral weight at high energies. The larger influence of the explicit solvent environment on the vibronic spectra of the GFP chromophores can be explained by the fact that both water and methanol are hydrogen-bonding solvents, such that it is to be expected that the explicit solvent environment plays a key role. On the other hand, benzene and cyclohexane are non-polar solvents, whereas acetone is polar but aprotic, such that the solute-solvent interactions for Nile Red in the three chosen solvents is expected to be much weaker.

The results suggest that for any solvated system with strong solute-solvent interactions, the explicit solvent environment has to be explicitly accounted for when computing vibronic

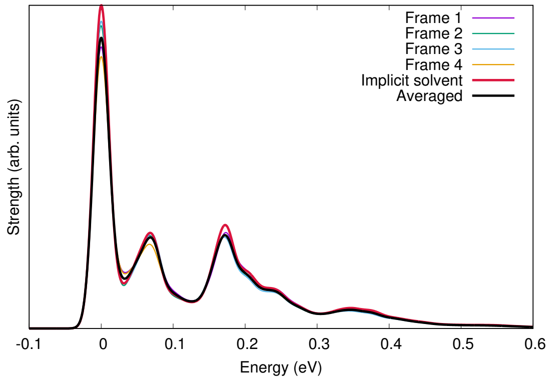


a) Nile Red in acetone

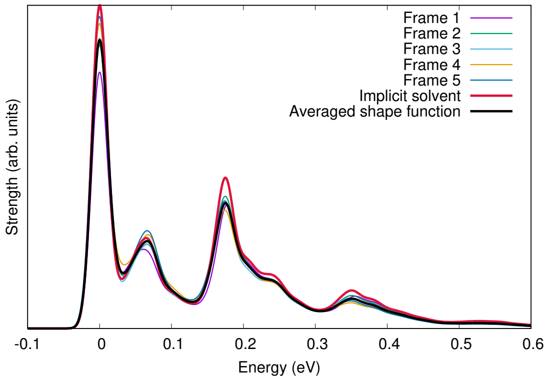


b) Nile Red in benzene

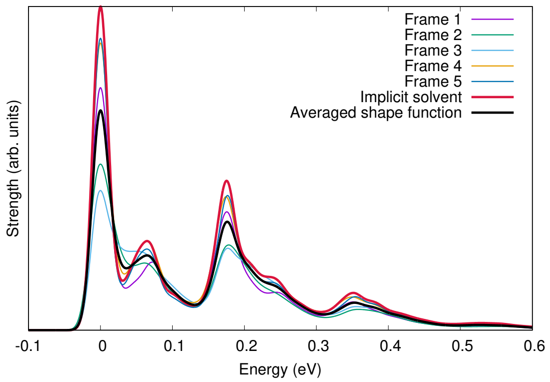


c) Nile Red in cyclohexane

FIG. 12: Vibronic shape functions for Nile Red in acetone, benzene, and cyclohexane, as calculated in implicit solvent as well as in frozen solvent environments taken from five uncorrelated MD snapshots. The vibronic shape function used to construct the absorption spectrum is the average of the vibronic spectra from the five individual frozen solvent snapshots and is also plotted for comparison. All spectra are shifted such that the 0-0 peak is at 0 eV. A Gaussian broadening with $\sigma = 0.0105$ eV is applied to all shape functions.

spectra.

## IV. STANDARDIZED MOMENTS OF THE DISTRIBUTION OF VERTICAL EXCITATION ENERGIES

In this section we analyze the computed vertical excitation energies in more detail. In each case, we focus on the bright $S_1$ state only and ignore variations in oscillator strength.

In particular, we are interested in quantifying the degree to which the distribution of $S_1$ excitation energies deviates from that of a normal distribution. This can be achieved by studying the higher order standardized moments of the distributions in question. Here, we focus on the skewness $\gamma_1$ and excess kurtosis $\gamma_2$ that, for a set of random variables $\{x_i\}$ with mean $\mu$ and standard deviation $\sigma$, are defined as

$$\gamma_1 = \frac{\sum_i^N (x_i - \mu)^3 / N}{\sigma^3} \tag{1}$$

$$\gamma_2 = \frac{\sum_i^N (x_i - \mu)^4 / N}{\sigma^4} - 3 \tag{2}$$

The excess kurtosis is a useful measure as the kurtosis of a normal distribution is equal to 3, such that its excess kurtosis is equal to zero. Roughly speaking, skewness provides a measure of asymmetry of the distribution, while excess kurtosis measures the heaviness of the tails of the distribution.

The two measures can be combined in a single test to determine whether a given data set is likely to be drawn from a normal distribution. Here, we make use of the D'Agostino-Pearson[21] test. The test returns a $p$-value that can be taken as a measure of confidence in rejecting the null-hypothesis that the data set was drawn from an underlying normal distribution.

Measures of skewness, excess kurtosis, as well as the $p$-value of the D'Agostino-Pearson test for normality for all sets of vertical excitation energies produced in this work can be found in Table I. We first notice that all data sets show a positive skew, meaning a tendency to form longer tails in the high energies than the low energies. Furthermore, Nile Red in benzene and Nile Red in acetone show very pronounced excess kurtosis, meaning a strong tendency towards heavy tails in the distribution of excitation energies.

From the $p$-values that are produced by the D'Agostino-Pearson test, it follows that the distributions of Nile Red in all solvents are very strongly non-Gaussian, whereas for the solvated GFP chromophores there is good evidence that the underlying distribution is non-Gaussian. Most interesting however is the analysis of the distribution of energies for the calculations where Nile Red is kept frozen in its ground state structure and only the solvent degrees of freedom are sampled over. Since the solute is kept frozen, all influence on the on the excitation energies originates from solvent conformations, and can be characterized by short-range polarization effects in the first solvation shell and long-range electrostatic interactions. In cases where direct solute-solvent interactions are weak, the influence of the

| System | Skew | Excess Kurtosis | $p$-value |
|---|---|---|---|
| GFP anion water | 0.184 | 0.234 | 0.0005 |
| GFP neutral+ methanol | 0.110 | 0.285 | 0.0078 |
| Nile Red Acetone | 0.526 | 3.218 | $1.6{\times}10^{-52}$ |
| Nile Red Benzene | 0.384 | 1.429 | $8.7\ {\times}10^{-25}$ |
| Nile Red Cyclohex. | 0.266 | 0.379 | $1.0{\times}10^{-17}$ |
| Frozen solute Acetone | 0.137 | -0.302 | 0.149 |
| Frozen solute Benzene | 0.308 | 0.339 | 0.0063 |
| Frozen solute Cyclohex. | 0.197 | 0.005 | 0.193 |

TABLE I: Analysis of the distribution of vertical excitation energies of the bright $S_1$ state for all systems studied in this work. The first two columns report the standardized skewness and excess kurtosis of the individual data sets, while the third column reports the $p$-value for the D'Agostino-Pearson omnibus test that is used as a measure of departure of the data set from the normal distribution.

solvent on the excitation energy of the solute is often assumed to be Gaussian in nature[22]. However, regarding our results obtained, it becomes clear that the frozen solute calculations in acetone and cyclohexane produce sets of vertical excitation energies that are consistent with underlying Gaussian statistics, but there is good evidence that the energies for the frozen solute in benzene do not follow Gaussian statistics. This finding can be straightforwardly interpreted by considering that acetone and cyclohexane do not interact strongly with Nile Red, whereas aromatic solvents like benzene and toluene have a tendency to form $\pi$-stacking conformations, meaning that the first solvation shell is highly ordered[3]. Thus even in systems where we artificially decouple the motion of the solute and the solvent by keeping the solute frozen, the vertical excitation energies only follow an underlying Gaussian statistic if there are no significant solute-solvent interactions and all influence of solvent conformations on the excitation energy is essentially due to electrostatics.

## V. INFLUENCE OF THE CHOICE OF SHAPE FUNCTION ON COMPUTED SPECTRA

As demonstrated in Section IIID, the local explicit solvent environment produces a significant amount of variability between the vibronic shape functions of different frozen solvent snapshots for the GFP chromophores and nile red in cyclohexane, while shape functions for nile red in acetone and benzene seem to be largely independent of the solvent environment. The observed variability of shape functions means that the assumption of a single average vibronic shape function for all solute-solvent conformations can only hold approximately in these systems. Furthermore, we note that in cases there is a large amount of variability in the shape functions, averaging over only $N_{\text{shape}} = 5$ might not yield a converged representation of the average shape function in the given system. It is therefore vital to test how sensitive the computed absorption spectra are with respect to the choice of vibronic shape function.

To do so, we take nile red in cyclohexane and the GFP anion in water and compute the vibronically broadened absorption spectra. However, rather than taking the average vibronic shape function, we use two different shape functions taken from the $N_{\text{shape}}$ frozen solvent conformations. For the GFP anion we use the shape functions of Frame 1 and Frame 3, while for nile red in cyclohexane we take Frame 3 and Frame 5, as these frames correspond to the shape functions that differ the most and are thus expected to yield the maximum changes in the spectrum.

The results for both systems can be found in Fig. 13. We note that in the case of the GFP anion in water, the Frame 1 shape function yields a somewhat broader absorption spectrum than the Frame 3 shape function. This is due to the fact that the Frame 1 shape function shows a large redistribution of spectral weight from the 0-0 transitions to higher energy. For the nile red chromophore in cyclohexane however, both shape functions produce almost identical vibronic spectra. It can therefore be concluded that despite the variability of shape functions in the case of nile red in cyclohexane, the use of an average vibronic shape function is likely to be valid in this system, as the observed variability only introduces minor changes to the computed vibronic absorption spectrum. The GFP anion results are more sensitive to the observed variability in the vibronic shape functions and an average shape function approach is a slightly less good approximation for this system. However, we note that the

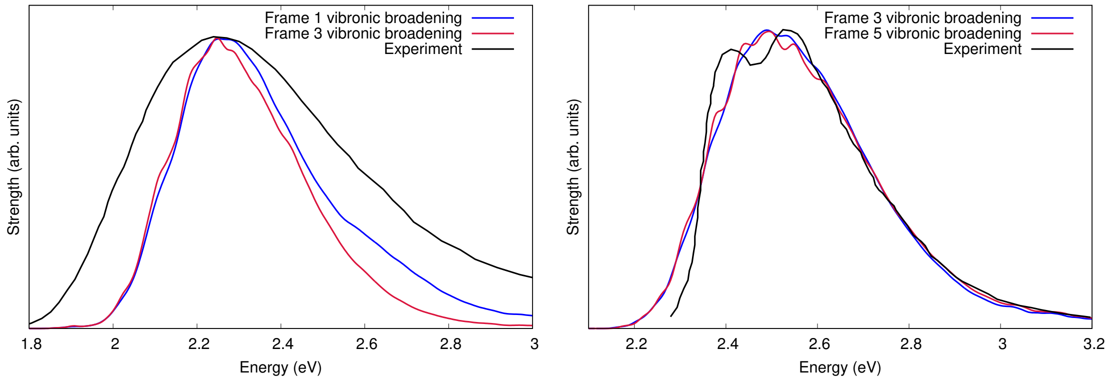


a) GFP anion in water    b) Nile Red in cyclohexane

FIG. 13: Vibronically broadened spectra for the GFP anion in water and Nile Red in cyclohexane and cyclohexane, as calculated using the vibronic shape functions of two different explicit frozen solvent conformations. The two snapshots are chosen such that the difference between the the shape functions used to create the spectra is maximized. All spectra are scaled and shifted in order to align with the experimental results.

GFP anion in water presents an example of a semi-flexible system with strong solute-solvent interactions and is thus expected to be a very difficult system to treat with the method proposed in this work. The fact that induced changes in the absorption spectra for extremal vibronic shape funtions are relatively moderate, it is likely that a treatment involving an averaged shape function is still valid in this system to a relatively good approximation.

Finally, the fact that the observed variability of the shape function for nile red in cyclohexane only causes very minor changes to the spectrum can be seen as strong evidence that the origin of the failure to reproduce the double peak structure in this system is not due to inaccuracies in the vibronic shape functions. Rather, the likely source of error is the MD sampling of solute-solvent conformations, which seems to produce a distribution of excitation energies that lacks the very sharp absorption onset seen experimentally.


[1] D. A. Case, D. S. Cerutti, T. E. Cheatham, III, T. A. Darden, R. E. Duke, T. J. Giese, H. Gohlke, A. W. Goetz, D. Greene, N. Homeyer, S. Izadi, A. Kovalenko, T. S. Lee, S. LeGrand, P. Li, C. Lin, J. Liu, T. Luchko, R. Luo, D. Mermelstein, K. M. Merz, G. Monard, H. Nguyen, I. Omelyan, A. Onufriev, F. Pan, R. Qi, D. R. Roe, A. Roitberg, C. Sagui, C. L. Simmerling,

W. M. Botello-Smith, J. Swails, R. C. Walker, J. Wang, R. M. Wolf, X. Wu, L. Xiao, D. M. York and P. A. Kollman (2017), AMBER 2017, University of California, San Francisco.

[2] W. L. Jorgensen, J. Chandrasekhar, and J. D. Madura, *"Comparison of simple potential functions for simulating liquid water"*, J. Chem. Phys. **79**, 926 (1983).

[3] T. J. Zuehlsdorff, P. D. Haynes, M. C. Payne, and N. D. M. Hine, *"Predicting solvatochromic shifts and colours of a solvated organic dye: The example of Nile Red"*, J. Chem. Phys. **146**, 124504 (2017).

[4] W. Humphrey, A. Dalke, and K. Schulten, *"VMD - Visual Molecular Dynamics"*, J. Molec. Graphics, **14**, 33-38 (1996).

[5] Gaussian Development Version, Revision I.09, M. J. Frisch, G. W. Trucks, H. B. Schlegel, G. E. Scuseria, M. A. Robb, J. R. Cheeseman, G. Scalmani, V. Barone, G. A. Petersson, H. Nakatsuji, X. Li, M. Caricato, A. V. Marenich, J. Bloino, B. G. Janesko, R. Gomperts, B. Mennucci, H. P. Hratchian, J. V. Ortiz, A. F. Izmaylov, J. L. Sonnenberg, D. Williams-Young, F. Ding, F. Lipparini, F. Egidi, J. Goings, B. Peng, A. Petrone, T. Henderson, D. Ranasinghe, V. G. Zakrzewski, J. Gao, N. Rega, G. Zheng, W. Liang, M. Hada, M. Ehara, K. Toyota, R. Fukuda, J. Hasegawa, M. Ishida, T. Nakajima, Y. Honda, O. Kitao, H. Nakai, T. Vreven, K. Throssell, J. A. Montgomery, Jr., J. E. Peralta, F. Ogliaro, M. J. Bearpark, J. J. Heyd, E. N. Brothers, K. N. Kudin, V. N. Staroverov, T. A. Keith, R. Kobayashi, J. Normand, K. Raghavachari, A. P. Rendell, J. C. Burant, S. S. Iyengar, J. Tomasi, M. Cossi, J. M. Millam, M. Klene, C. Adamo, R. Cammi, J. W. Ochterski, R. L. Martin, K. Morokuma, O. Farkas, J. B. Foresman, and D. J. Fox, Gaussian, Inc., Wallingford CT, 2016.

[6] A. D. Becke, *"Density-functional thermochemistry. III. The role of exact exchange"*, J. Chem. Phys. **98**, 5648 (1993).

[7] I.S. Ufimtsev and T. J. Martínez, *"Quantum Chemistry on Graphical Processing Units. 3. Analytical Energy Gradients and First Principles Molecular Dynamics"*, J. Chem. Theory Comput. **5**, 2619 (2009).

[8] A. V. Titov, I. S. Ufimtsev, N. Luehr, and T. J. Martínez, *"Generating Efficient Quantum Chemistry Codes for Novel Architectures"*, J. Chem. Theory Comput. **9**, 213 (2013).

[9] T. Yanai, D. P. Tew, and N. C. Handy, *"A new hybrid exchange-correlation functional using the Coulomb-attenuating method (CAM-B3LYP)"*, Chem. Phys. Lett. **393**, 51 (2004).

[10] A. L. Fetter, and J. D. Walecka, *"Quantum Theory of Many-Particle Systems"* (McGraw-Hill,

New York, 1971).

[11] S. Hirata, and M. Head-Gordon, *"Time-dependent density functional theory within the Tamm-Dancoff approximation"*, Chem. Phys. Lett. **314**, 291-299 (1999).

[12] E. Epifanovsky, I. Polyakov, B. Grigorenko, A. Nemukhin, and A. I. Krylov, *"Quantum Chemical Benchmark Studies of the Electronic Properties of the Green Fluorescent Protein Chromophore. 1. Electronically Excited and Ionized States of the Anionic Chromophore in the Gas Phase"*, J. Chem. Theory Comput. **5**, 1895-1906 (2009).

[13] M. D. Davari, F. J. Avila Ferrer, D. Morozov, F. Santoro, and G. Groenhof, *"The Lineshape of the Electronic Spectrum of the Green Fluorescent Protein Chromophore, Part I: Gas Phase"*, Chem. Phys. Chem. **15**, 3236-3245 (2014).

[14] C. A. Guido, B. Mennucci, D. Jacqueminc, and C. Adamo, *"Planar vs. twisted intramolecular charge transfer mechanism in Nile Red: new hints from theory"*, Phys. Chem. Chem. Phys. **12**, 8016 (2010).

[15] A.Y. Freidzon, A. A. Safonov, A. A. Bagaturyants, and M. V. Alfimov, *"Solvatofluorochromism and Twisted Intramolecular Charge-Transfer State of the Nile Red Dye"*, Int. J. Quantum Chem. **112**, 3059-3067 (2012).

[16] J.-D. Chai and M. Head-Gordon, *"Systematic optimization of long-range corrected hybrid density functionals"*, J. Chem. Phys. **128** , 084106 (2008).

[17] F. Santoro, R. Improta, A. Lami, J. Bloino, and V. Barone, *"Effective method to compute Franck-Condon integrals for optical spectra of large molecules in solution"*, J. Chem. Phys. **126**, 169903 (2007).

[18] F. Santoro, FCclasses: A Fortran 77 Code; 2008. (available via the Internet at http://www.pi.iccom.cnr.it/fcclasses; last accessed 11/07/2017).

[19] F. Santoro, R. Improta, A. Lami, and V. Barone, *"An effective method to compute vibrationally resolved optical spectra of large molecules at finite temperature in the gas-phase and in solution"*, J. Chem. Phys. **126**, 184102 (2007).

[20] S. Grimme, J. Antony, S. Ehrlich, and H. Krieg, *"A consistent and accurate ab initio parameterization of density functional dispersion correction (DFT-D) for the 94 elements H-Pu"*, J. Chem. Phys. **132**, 154104 (2010).

[21] R. B. D'Agostino, A. Berlanger, and R. B. D'Agostino, Jr., *"A suggestion for using powerful and informative tests of normality"*, Am. Stat. **44** (4), 316?321 (1990).

[22] J. Cerezo, F. J. Avila Ferrer, G. Prampolini, and. F. Santoro, *“Modeling Solvent Broadening on the Vibronic Spectra of Coumarin Dyes. From Implicit to Explicit Solvent Models”*, J. Chem. Theory Comput. **11**, 5810-5825 (2015).
